# Supplementary material for: AEGIS: A Holistic Benchmark for Evaluating Forensic Analysis of AI-Generated Academic Images
Source: arXiv:2604.28177 source file (2026-05-21)
Supplement: Supplementary file 1 [file 1_experiment_expert.tex]

\begin{table*}[t]
\small
\centering
\setlength{\tabcolsep}{4pt}

\begin{tabularx}{\linewidth}{X | cc c cc  cc}
\toprule
\multirow{3}{*}{\textbf{Models}} & 
\multicolumn{5}{c|}{\textbf{Forgery Scope Discrimination}} & 
\multicolumn{2}{c}{\textbf{Tampering Pinpointing}} \\
\cmidrule(lr){2-6} \cmidrule(lr){7-8}
& \multirow{2}{*}{\textbf{ACC}} 
& \multirow{2}{*}{\textbf{M-F1}} 
& \multirow{2}{*}{\textbf{Real-F1}} 
& \multicolumn{2}{c}{\textbf{Forgery-F1}} 
& \multirow{2}{*}{\textbf{IoU}} 
& \multirow{2}{*}{\textbf{Pixel-F1}} \\
\cmidrule(lr){5-6}
& & & & \textbf{Entire-F1} & \textbf{Partial-F1} & & \\
\midrule

% --- Vision-Only Expert Models ---
\multicolumn{8}{l}{\textit{\textbf{Vision-Only Expert Models (Detection-Only)}}} \\
\midrule
DRCT & 55.05 & 39.55 & 14.15 & \multicolumn{2}{c}{64.95} & -- & -- \\
DIRE & 58.16 & 50.41 & 30.79 & \multicolumn{2}{c}{70.02} & -- & -- \\
AIDE & 79.54 & 44.74 & 0.85 & \multicolumn{2}{c}{88.63} & -- & -- \\
AlignedForensics & 47.57 & 42.48 & 25.37 & \multicolumn{2}{c}{59.59} & -- & -- \\
Denoising Trajectory & 73.68 & 65.37 & 48.40 & \multicolumn{2}{c}{82.33} & -- & -- \\
DDA & 74.19 & 67.07 & 51.75 & \multicolumn{2}{c}{82.38} & -- & -- \\

% --- Hybrid / MLLM-Assisted Expert Models ---
\midrule
\multicolumn{8}{l}{\textit{\textbf{Hybrid MLLM-Assisted Expert Models}}} \\
\midrule
FakeShield & 59.72 & 62.08 & 44.73 & \multicolumn{2}{c}{79.42} & 30.09 & 69.11 \\
SIDA & 52.91 & 64.38 & 87.82 & 62.43 & 42.89 & 3.66 & 54.28 \\
FakeVLM & 58.73 & 55.39 & 43.17 & \multicolumn{2}{c}{67.60} & -- & -- \\

\bottomrule
\end{tabularx}
\caption{Performance comparison of expert model.}
\label{tab:experiment_expert}
\end{table*}
